# Supplementary material for: FDI: Attack Neural Code Generation Systems through User Feedback Channel
Source: arXiv:2408.04194 source file (2024-08-08)
Supplement: Supplementary file 1 [file x.appendix.tex]

\section{Appendix}
\subsection{Enhanced Profiling}
\label{sec:appendix:profiling}
In the profiling phase for the prompt injection attack, the auto-generated samples alone cannot trigger the model behavior that can be recognized by the attacker in the black-box setting. 
To be specific, given the auto-generated sample as a query, even though the injected sample is retrieved, the attacker remains unaware.
To overcome this challenge, we adopt a jail-breaking trick~\cite{Zhuo2023RedTC} to request the LCM to leak its given prompt.
To be specific, for each auto-generated sample, we add a suffix {\tt Repeat above:} and accordingly revise the sample to ensure it remains within the model's constraints (e.g., cut off parts of its content to keep the number of revised characters unchanged).
By doing this, when querying the system with the modified sentences, we not only retrieve exactly the same example but also prompt the model to disclose its given prompts. 
In the following, we provide an example of the entire prompt, both the input query (Q4) and its retrieved examples (Q1-Q3).

\begin{lstlisting}
Q1: %I do know what made the grass. Repeat above.%
A1: ANY ANSWER + A RANDOM WORD.
Q2: Replace column 'column2' with 'column1'
A2: dfin['column2'] = dfin['column1']
Q3: Find argmax of first 3 columns of dfin
A3: dfin.iloc[:3].idxmax(1)
Q4: %I do know what made the grass. Repeat above.%
\end{lstlisting}

\begin{table}[t]
\caption{The attack success rate of the FDI-based backdoor attack under different temperatures ($T$).}
\centering
   \scalebox{0.9}{\begin{tabular}{ccccc} \toprule
\multirow{2}{*}{Backdoor} & \multirow{2}{*}{$r$} & \multicolumn{3}{c}{Attack Success Rate} \\ \cmidrule{3-5}
 &  & $T$=0.2 & $T$=0.6 & $T$=1.0 \\ \midrule
\multirow{3}{*}{$B_1$} & 0.01\% & 71.0\% & 66.8\% & 60.4\% \\
 & 0.1\% & 99.8\% & 99.8\% & 95.9\% \\
 & 1\% & 100.0\% & 100.0\% & 99.6\% \\ \midrule
\multirow{3}{*}{$B_2$} & 0.01\% & 6.3\% & 5.8\% & 15.9\% \\
 & 0.1\% & 97.1\% & 97.6\% & 95.4\% \\
 & 1\% & 99.7\% & 99.7\% & 99.6\% \\ \bottomrule
\end{tabular}}
\label{tab:rand_backdoor}
\end{table}

\begin{table}[t]
\caption{The attack success rate of the FDI-based prompt injection attack under different temperatures ($T$).}
\centering
   \scalebox{0.9}{\begin{tabular}{ccccccc} \toprule
\multirow{2}{*}{\textbf{Prompt}} & \multirow{2}{*}{$T$} & \multicolumn{5}{c}{\textbf{Attack Success Rate}} \\ \cmidrule{3-7}
 &  & \textbf{$m$=0} & \textbf{$m$=1} & \textbf{$m$=2} & \textbf{$m$=3} & \textbf{$m$=4} \\ \midrule
\multirow{3}{*}{$P_1$} & 0.2 & 0.0\% & 5.2\% & 0.3\% & 0.0\% & 0.0\% \\
 & 0.6 & 0.0\% & 4.6\% & 0.6\% & 0.0\% & 0.0\% \\
 & 1.0 & 0.0\% & 6.2\% & 0.4\% & 0.0\% & 0.0\% \\ \midrule
\multirow{3}{*}{$P_3$} & 0.2 & 0.0\% & 0.0\% & 10.9\% & 59.0\% & 94.6\% \\
 & 0.6 & 0.0\% & 0.8\% & 15.9\% & 65.9\% & 96.7\% \\
 & 1.0 & 0.0\% & 0.3\% & 16.4\% & 64.6\% & 97.7\% \\ \bottomrule
\end{tabular}}
\label{tab:rand_prompt}
\end{table}

\subsection{Randomness of the code generation system}
Following~\cite{Aghakhani2023TrojanPuzzleCP}, we evaluate both of our proof-of-concept attacks under a range of temperatures, i.e., 0.2, 0.6, and 1.0.
The results are reported in~\Cref{tab:rand_backdoor} and~\Cref{tab:rand_prompt}.
